# Supplementary material for: Benchmarking Popular Classification Models' Robustness to Random and Targeted Corruptions
Source: arXiv:2002.00754 source file (2020-01-31)
Supplement: Supplementary file 1 [file appendix.tex]

\begin{table}[t]
\small
\begin{tabular}{llllll}
\hline
\textbf{Algorithm} & \textbf{Character Changed} & \textbf{SST2} & \textbf{IMDB} & \textbf{YELP} & \textbf{DBPEDIA} \\
\hline
\hline
multirow{2}{*}{\textbf{Baseline}} & & 86.7 & 87.3 & 93.1 & 96.7 \\
\hline
\hline
\multirow{2}{*}{\textbf{Duplication Ch}} & Random & 82.01 & 85.15 & 90.40 & 93.72 \\
 & First & 82.01 & 85.13 & 93.39 & 93.75 \\
 \hline
\multirow{2}{*}{\textbf{Adjacent Ch}} & Random & 82.01  & 85.15 & 90.42 & 93.72 \\
 & First  & 82.07 & 85.13 & 90.04 & 93.71 \\
 \hline
\multirow{2}{*}{\textbf{Near Ch}} & Random & 82.14 & 85.13 & 90.37 & 93.72 \\
 & First  & 82.01 & 85.13 & 90.33 & 93.71 \\
 \hline
 \multirow{2}{*}{\textbf{Missing Ch}} & Random & 81.77 & 85.12 & 90.30 & 93.73 \\
 & First  & 81.77 & 85.06 & 90.37 & 93.71 \\
 \hline
\multicolumn{1}{c}{\multirow{2}{*}{\textbf{Homophones}}} & Random & 85.99 & 85.47 & 91.58 & 95.90 \\
\multicolumn{1}{c}{} & First  & 85.99 & 85.48 & 91.60 & 95.90 \\
\hline
\end{tabular}
\caption{Accuracies on the FastText model for all datasets after introducing different type of typographical errors in 3 words in a test case}
\end{table}

\begin{table}[t]
\small
\begin{tabular}{llllll}
\hline
\textbf{Algorithm} & \textbf{Character Changed} & \textbf{SST2} & \textbf{IMDB} & \textbf{YELP} & \textbf{DBPEDIA} \\
\hline
\hline
multirow{2}{*}{\textbf{Baseline}} & & 86.7 & 87.3 & 93.1 & 96.7 \\
\hline
\hline
\multirow{2}{*}{\textbf{Duplication Ch}} & Random & 80.49 & 84.78 & 89.73 & 91.40 \\
 & First & 80.49 & 84.79 & 89.68 & 91.52 \\
 \hline
\multirow{2}{*}{\textbf{Adjacent Ch}} & Random & 80.49  & 84.76 & 89.68 & 91.36 \\
 & First  & 80.56 & 84.74 & 89.64 & 91.35 \\
 \hline
\multirow{2}{*}{\textbf{Near Ch}} & & Random & 80.49  & 84.77 & 89.64 & 91.35 \\
 & First  & 80.36 & 84.77 & 89.44 & 91.36 \\
 \hline
 \multirow{2}{*}{\textbf{Missing Ch}} & Random & 80.22  & 84.79 & 89.64 & 91.43 \\
 & First  & 80.15 & 84.74 & 89.61 & 91.36 \\
 \hline
\multicolumn{1}{c}{\multirow{2}{*}{\textbf{Homophones}}} & Random & 85.49 & 85.38 & 91.50 & 95.85 \\
\multicolumn{1}{c}{} & First  & 85.42 & 85.38 & 91.51 & 95.85 \\
\hline
\end{tabular}
\caption{Accuracies on the FastText model for all datasets after introducing different type of typographical errors in 5 words in a test case}
\end{table}

\begin{table}[t]
\small
\begin{tabular}{llllll}
\hline
\textbf{Algorithm} & \textbf{Character Changed} & \textbf{SST2} & \textbf{IMDB} & \textbf{YELP} & \textbf{DBPEDIA} \\
\hline
\hline
multirow{2}{*}{\textbf{Baseline}} & & 86.7 & 87.3 & 93.1 & 96.7 \\
\hline
\hline
\multirow{2}{*}{\textbf{Emoji}} & Random & 82.07 & 85.21 & 90.48 & 93.71 \\
 & First & 82.07 & 85.21 & 90.48 & 93.71 \\
 \hline
\multirow{2}{*}{\textbf{Homoglyph}} & Random & 82.07  & 85.21 & 90.48 & 93.71 \\
 & First  & 82.07 & 85.21 & 90.48 & 93.71 \\
 \hline
\multirow{2}{*}{\textbf{Punctuation}} & Random & 82.07 & 85.21 & 90.56 & 93.88 \\
 & First  & 82.07 & 85.21 & 90.53 & 93.84 \\
 \hline
\multirow{2}{*}{\textbf{Random Ch}} & Random & 82.07 & 85.19 & 90.48 & 93.72 \\
 & First  & 82.07 & 85.21 & 90.48 & 93.74 \\
 \hline
\multirow{2}{*}{\textbf{Random Space}} & Random & 82.93 & 85.17 & 90.76 & 94.22 \\
 & First  & 86.36 & 85.57 & 90.05 & 95.98 \\
 \hline
\multirow{2}{*}{\textbf{Special Ch}} & Random & 82.07 & 85.21 & 90.48 & 93.71 \\
 & First  & 82.07 & 85.21 & 90.48 & 93.71 \\
 \hline
\multicolumn{1}{c}{\multirow{2}{*}{\textbf{Stop Words}}} & Random & 84.46 & 85.55 & 91.61 & 95.95 \\
\multicolumn{1}{c}{} & First  & 83.85 & 85.58 & 91.61 & 95.95 \\
\hline
\end{tabular}
\caption{Accuracies on the FastText model for all datasets after introducing different type of noise in 3  random words from a test case}
\end{table}

\begin{table}[t]
\small
\begin{tabular}{llllll}
\hline
\textbf{Algorithm} & \textbf{Character Changed} & \textbf{SST2} & \textbf{IMDB} & \textbf{YELP} & \textbf{DBPEDIA} \\
\hline
\hline
multirow{2}{*}{\textbf{Baseline}} & & 86.7 & 87.3 & 93.1 & 96.7 \\
\hline
\hline
\multirow{2}{*}{\textbf{Emoji}} & Random & 82.07 & 85.21 & 90.48 & 93.71 \\
 & First & 82.07 & 85.21 & 90.48 & 93.71 \\
 \hline
\multirow{2}{*}{\textbf{Homoglyph}} & Random & 82.07  & 85.21 & 90.48 & 93.71 \\
 & First  & 82.07 & 85.21 & 90.48 & 93.71 \\
 \hline
\multirow{2}{*}{\textbf{Punctuation}} & Random & 82.07 & 85.21 & 90.56 & 93.88 \\
 & First  & 82.07 & 85.21 & 90.53 & 93.84 \\
 \hline
\multirow{2}{*}{\textbf{Random Ch}} & Random & 82.07 & 85.19 & 90.48 & 93.72 \\
 & First  & 82.07 & 85.21 & 90.48 & 93.74 \\
 \hline
\multirow{2}{*}{\textbf{Random Space}} & Random & 82.93 & 85.17 & 90.76 & 94.22 \\
 & First  & 86.36 & 85.57 & 90.05 & 95.98 \\
 \hline
\multirow{2}{*}{\textbf{Special Ch}} & Random & 82.07 & 85.21 & 90.48 & 93.71 \\
 & First  & 82.07 & 85.21 & 90.48 & 93.71 \\
 \hline
\multicolumn{1}{c}{\multirow{2}{*}{\textbf{Stop Words}}} & Random & 84.46 & 85.55 & 91.61 & 95.95 \\
\multicolumn{1}{c}{} & First  & 83.85 & 85.58 & 91.61 & 95.95 \\
\hline
\end{tabular}
\caption{Accuracies on the FastText model for all datasets after introducing different type of noise in 5 random words from a test case}
\end{table}
